# Supplementary material for: Route to Time and Time to Route: Travel Time Estimation from Sparse Trajectories
Source: arXiv:2206.10418 source file (2022-06-21)
Supplement: Supplementary file 1 [file appendix.tex]

\clearpage
\appendix 
\setcounter{figure}{0}    
\setcounter{table}{0}
\setcounter{equation}{0}
